# Supplementary material for: Safe exploration in reproducing kernel Hilbert spaces
Source: arXiv:2503.10352 source file (2025-03-13)
Supplement: Supplementary file 1 [file probability_spaces.tex]

\section{Joint probability spaces and the law of total probability}\label{app:probability_spaces}

\tikzexternaldisable
% \todo[inline]{Use $\mathrm{C}$ instead of $\perp$ for complement sets.
% }
\tikzexternalenable
In this paper, and especially in the proof of Theorem~\ref{th:error_bound}, we apply the law of total probability to combine the uncertainties that arise from deriving confidence intervals (with known RKHS norm) with the uncertainty that comes from the RKHS norm over-estimation. 

In the following, we summarize the problem.
We define the following events for each iteration~$t$:
\begin{itemize}
    \item $\mathcal C_t$: The ground truth is contained in the confidence intervals.
    \item $\mathcal B_t$: The RKHS norm over-estimation is correct.
\end{itemize}

From, \eg Theorem~1 of \cite{chowdhury2017kernelized}, we can state that~$\mathbb P[\mathcal C_t\vert B_t]=1-\delta$. 
Crucially, the RKHS norm is a deterministic object in \cite{chowdhury2017kernelized}.
Thus, the authors state $\mathbb P[\mathcal C_t]\geq 1-\delta$ without conditioning on the event~$\mathcal B_t$.
In Theorem~\ref{th:error_bound}, we use the law of total probability to write
\begin{align*}
    \mathbb P[\mathcal C_t\vert \mathcal B_t] = \mathbb P[\mathcal C_t\vert \mathcal B_t]\cdot \mathbb P[\mathcal B_t] + \mathbb P[\mathcal C_t\vert \mathcal B_t^\mathrm{C}]\cdot \mathbb P[\mathcal B_t^\mathrm{C}] \geq \mathbb P[\mathcal C_t\vert \mathcal B_t]\cdot \mathbb P[\mathcal B_t].
\end{align*}
Then, we take~$\mathbb P[\mathcal C_t\vert \mathcal B_t]$ from, \eg \cite{chowdhury2017kernelized} or \cite{abbasi2013online} and~$\mathbb P[\mathcal B_t]$ from our results in Theorem~\ref{th:RKHS_scenario} and/or Corollary~\ref{co:RKHS_stop}.

\subsection{Why the law of total probability is not directly applicable}
The problem\footnote{%
Another potential problem can arise because $\mathbb P[\mathcal B_t^\mathrm{C}]=0$; zero probabilities in conditional probabilities can be problematic.
} 
is that we are connecting the uncertainty of two probability spaces, \ie we are combining~\emph{(i)} the herein introduced uncertainty on the RKHS norm
with~\emph{(ii)} the uncertainty on the confidence intervals.\footnote{%
The uncertainty on the confidence intervals are solely induced by (sub-Gaussian) measurement noise.
We follow the well-known confidence intervals construction from \cite{abbasi2013online}---as shown in Appendix~\ref{app:abbasi}.
We refer the reader to the proof of Theorem~1 in \cite{chowdhury2017kernelized} for bounding the norm of the accumulated measurement error and to Section~3.2 of \cite{abbasi2013online} to general vector-valued martingale tail inequalities.
}
Uncertainty~\emph{(i)} lives on the probability space $(\Omega_1, \mathcal F_1, \mathbb P_1)$ whereas uncertainty~\emph{(ii)} lives on the probability space $(\Omega_2, \mathcal F_2, \mathbb P_2)$.

\subsection{Why a product probability space is no (direct) remedy}

\paragraph{Uncertainty~\emph{(i)}}

We choose an equivalent construction of the probability space in which we use the scenario approach as \cite{romao2022exact}.
Specifically, each random RKHS function is a sample from the probability space $(\Omega_1, \mathcal F_1, \mathbb P_1)$.
We work with~$m$ random RKHS functions and, since the random RKHS functions are i.i.d.\ samples, the \emph{product probability space} (see, \eg Appendix~3.1 in \cite{Steinwart2008SVM}) $(\Omega_1^m, \otimes_{i=1}^m \mathcal F_1, \mathcal P_1^m)$ provides a natural (new) probability space.

\begin{remark}[Product probability spaces]\label{re:product}
    The fact that the random RKHS functions are independent is indispensable because the construction of product probability spaces is based on~$\Omega_1^m$ being an $m$-dimensional rectangle and each instance of an event~$E_i\in\Omega_1$ with $(E_1,\ldots,E_m)\in\Omega_1^m$ is a set in dimension~$i$ of the $m$-dimensional rectangle.
Naturally, an intersection between these sets, \ie dependence between random variables and events, cannot be represented with product probability spaces. 
\end{remark}

We map the probability space to a simpler and more interpretable but for our needs equivalent probability space.
Instead of working on the sample space~$\Omega_1^m$ that is the Cartesian product of spaces from which the random RKHS functions are sampled, we work with events:
\begin{itemize}
    \item $\mathcal B_t:$ The RKHS norm over-estimation is correct, \ie $B\geq \|f\|_k$;
    \item $\mathcal B_t^\mathrm{C}:$ RKHS norm over-estimation is incorrect, \ie $B< \|f\|_k$.
\end{itemize}

Note that the event-based sample space and the $\sigma$-algebra are instances from the original sample space and $\sigma$-algebra. 
The events show a more interpretable version of the original probability space.
However, since the events can be equivalently represented in the old and new setting, we can use the original probability measure~$\mathbb P^m_1$ and obtain the probability space $(\{\mathcal B, \mathcal B^\mathrm{C}\}, 2^{\{\mathcal B, \mathcal B^\mathrm{C}\}}, \mathbb P_2^m)$, with $2^{\{\mathcal B, \mathcal B^\mathrm{C}\}}=\{\emptyset, \mathcal B, \mathcal B^\mathrm{C}, \{\mathcal B, \mathcal B^\mathrm{C}\}\}.$
In this discrete probability space, the probability measure is given by the tabular mapping
\begin{align*}
    \mathbb P_1^m[\{\mathcal B, \mathcal B^\mathrm{C}\}] &= 1 \\
    \mathbb P_1^m[\emptyset] &= 0 \\
    \mathbb P_1^m[\mathcal B] &=  1-\gamma \\
    \mathbb P_1^m[\mathcal B^\mathrm C] &= \gamma, 
\end{align*}
where the first two results follow from the definition of valid probability measures, the third equality follows from Theorem~\ref{th:RKHS_scenario}, while the final equality follows from the fact that $\mathbb P_1^m[\{\mathcal B, \mathcal \mathcal \mathcal B^\mathrm{C}\}]=\mathbb P_1^m[\mathcal B]+\mathbb P_1[\mathcal B^\mathrm{C}]$ since~$\mathcal B$ and~$\mathcal B^\mathrm{C}$ are disjoint.
\tikzexternaldisable
% \todo[inline]{I have ignored the double probability now in the PAC bounds. Might that be a problem? I do not think so; can we still state it with confidence?
% }
\tikzexternalenable

\paragraph{Uncertainty~\emph{(ii)}}

% \tikzexternaldisable
% \todo[inline]{Also still cleanly write down the original probability space of \cite{chowdhury2017kernelized} and/or \cite{abbasi2013online}.
% }
% \tikzexternalenable

We form an equivalent probability space transformation as we did for Uncertainty~\emph{(i)} instead of working on the original probability space $(\Omega_2, \mathcal F_2, \mathbb P_2)$.
On this probability space, \cite{chowdhury2017kernelized} and/or \cite{abbasi2013online} derive confidence intervals where the RKHS norm is a deterministic object.
The uncertainty solely arises from the sub-Gaussian measurement noise.
Specifically, the uncertainty arises bounding the norm of the accumulated measurement noise with respect to a positive definite matrix. 

First, we define the events
\begin{itemize}
    \item $\mathcal C_t$ The ground truth is contained in the confidence intervals.
    \item $\mathcal C_t^\mathrm C$ The ground truth is not contained in the confidence intervals.
\end{itemize}
The $\sigma$-algebra is again the power set of the sample space, \ie $2^{\{\mathcal C_t,\mathcal C_t^\mathrm{C}\}}=\{\{\mathcal C_t, \mathcal C_t^\mathrm{C}\},\mathcal C_t,\mathcal C_t^\mathrm{C},\emptyset\}$.
We take the same probability measure as in the original probability space and have
\begin{align*}
    \mathbb P_2[\{\mathcal C_t, \mathcal C_t^\mathrm{C}\}] &= 1 \\
    \mathbb P_2[\emptyset] &= 0 \\
    \mathbb P_2[\mathcal C_t] &=  1-\delta \\
    \mathbb P_2[\mathcal C_t^\mathrm C] &= \delta.
\end{align*}

\paragraph{Constructing a product probability space}
Now, as described in Appendix~3.1 of \cite{Steinwart2008SVM} or applied in \cite{romao2022exact}, we build a product probability space between the probability spaces induced by the aforementioned uncertainties~\emph{(i)} and~\emph{(ii)}.
The sample space of the new probability space is
\begin{align*}
\{\mathcal B,\mathcal B^\mathrm{C}\} \times \{\mathcal C,\mathcal C^\mathrm{C}\},
\end{align*}
while the $\sigma$-algebra is given by
\begin{align*}
    2^{\{\mathcal B,\mathcal B^\mathrm{C}\} \times \{\mathcal C,\mathcal C^\mathrm{C}\}}
\end{align*}
and the probability measure is
\begin{align*}
\mu \coloneqq \mathbb P_1^m \otimes \mathbb P_2,
\end{align*}
with $ \mathbb P_1^m \otimes \mathbb P_2(\mathcal B_t \times \mathcal C_t)= \mathbb P_1^m(\mathcal B_t)\cdot \mathbb P_2(\mathcal C_t)$ through the basic definition and construction of product probability spaces.

However, as described in Remark~\ref{re:product}, product probability spaces can only be used for disjoint probability spaces. 
As the RKHS norm affects the confidence intervals, these two probability spaces are not disjoint and the two random variables are not independent.

\begin{remark}[Addendum to Remark~\ref{re:product}]
    Consider an arbitrary probability space $(\Omega,\mathcal F, \mathbb P)$.
    If the product probability space construction could be used for intersecting probability spaces, then we could use the special case of both probability spaces being identical, leading to
    \begin{align*}
        \mathbb P \otimes \mathbb P (A \times B)=\mathbb P(A)\cdot \mathbb P(B), \quad \forall A,B \in \mathcal F.
    \end{align*}
That is, we would have
\begin{align*}
    \mathbb P[A \cap B] = \mathbb P [A] \cdot \mathbb P[B], \quad \forall A,B \in \mathcal F.
\end{align*}
However, it is well-known that this only holds if, and only if,~$A$ and~$B$ are independent events, \ie disjoint sets.
\end{remark}

\subsection{Trivial solution through detaching aleatoric and epistemic uncertainty}\label{app:trivial}
Uncertainty~\emph{(ii)} is quantified in, \eg, Theorem~2 in \cite{chowdhury2017kernelized}.
The proof of Theorem~2 in \cite{chowdhury2017kernelized} only contains deterministic steps and inserts the probabilistic upper bound on the norm of the accumulated noise that is derived in Theorem~1 of \cite{chowdhury2017kernelized}.
\tikzexternaldisable
% \todo[inline]{Just taking \cite{chowdhury2017kernelized} because I know the proof a bit better than \cite{abbasi2013online}; but totally equivalent in the arguments.}
\tikzexternalenable

Following the proof of Theorem~1 of \cite{chowdhury2017kernelized}, we have
\begin{align*}
M_t &= \frac{1}{\sqrt{(2\pi)^t\det(K_t+\sigma I)}} \int_{\mathbb R^t}\left(
\epsilon_{1:t}^\top\lambda -\frac{\|\lambda\|^2}{2}-\frac{\|\sigma\|_{(K_t+\sigma I)^{-1}}}{2}d\lambda
    \right) \\
    &=\ldots \\
    &= \frac{1}{\sqrt{\det(I+K_t+\sigma I)}}\exp\left(
\frac{1}{2}\|\epsilon_{1:t}\|_{(I+(K_t+\sigma I)^{-1})^{-1}}.
    \right).
\end{align*}
Therefore, we have
\begin{align*}
    \|\epsilon_{1:t}\|_{(I+(K_t+\sigma I)^{-1})^{-1}} = 2\ln
    \left(
\sqrt{\det(I+K_t+\sigma I)} M_t.
    \right)
\end{align*}
Since~$\mathbb E[M_\tau]\leq 1$, Markov's inequality gives
\begin{align*}
    \mathbb P_2\left[M_\tau> \frac{1}{\delta}\right] \leq \delta,
\end{align*}
for all~$\delta\in(0,1).$
Combining the last two results yields
\begin{align*}
    \mathbb{P}_2\left[
    \|\epsilon_{1:\tau}\|^2_{((K_\tau+\eta I)^{-1}+I)^{-1}}>2\ln\left(
    \sqrt{
\det((1+\eta)I)+K_\tau
    }/\delta
    \right)
    \right]
    =\mathbb P_2[M_\tau>1/\delta]\leq \delta
\end{align*}
for all $\delta\in(0,1)$.
Then, \cite{chowdhury2017kernelized} use a classic stopping-time criterion to prove that
\begin{align}\label{eq:noise_bound}
    \mathbb{P}_2\left[
\|\epsilon_{1:\tau^\prime}\|^2_{((K_{\tau^\prime}+\eta I)^{-1}+I)^{-1}}>2\ln\left(
    \sqrt{
\det((1+\eta)I)+K_{\tau^\prime}
    }/\delta
    \right)
    \right] \leq \delta
\end{align}
for all $\tau^\prime < \infty$.
Note that this probability was formulated according to the probability measure~$\mathbb P_2$.

Elementary computations in the proof of Theorem~2 of \cite{chowdhury2017kernelized} show that
\begin{align*}
    \lvert f(x)-k_t(x)^\top(K_t+\lambda I)^{-1}f_{1:t}\rvert \leq \|f\|_k \sigma_t(x),
\end{align*}
where~$\sigma_t(\cdot)$ the posterior GP standard deviation.\footnote{%
Note that the approximating function on the left-hand side is the kernel interpolating function, \ie it is the function in the pre-RKHS spanned by the kernel~$k$ on support points $x_{1:t}$ that interpolated all $(x_{1:t},f_{1:t})$ with the minimal RKHS norm.
}

Since this equation is deterministic, we can insert the herein developed statistical over-estimation of the RKHS norm~$B_t$ into the inequality, which we developed with respect to the probability measure~$\mathbb P^m$ (see Theorem~\ref{th:error_bound} and Corollary~\ref{co:RKHS_stop}). 
Since
\begin{align}\label{eq:uncertainty_1}
    \mathbb{P}_1^m\left[
B_t\geq \|f\|_k
    \right] \geq 1-\gamma,
\end{align}
we can state that
\begin{align}
    \mathbb{P}_1^m\left[
\lvert f(x)-k_t(x)^\top(K_t+\lambda I)^{-1}f_{1:t}\rvert \leq B_t \sigma_t(x)
    \right] \geq 1-\gamma
\end{align}
by combining the noise-free steps of \cite{chowdhury2017kernelized} with the proposed PAC RKHS norm over-estimation in Theorem~\ref{th:RKHS_scenario}.

Furthermore, we follow \cite{chowdhury2017kernelized} and replace the kernel interpolation function by the GP mean for which 
\begin{align*}
    \lvert f(x)-\mu_t(x)\rvert \leq
(\|f\|_k+\|\epsilon_{1:t}\|_{((K_{t}+\eta I)^{-1}+I)^{-1}}) \cdot \sigma_t(x)
\end{align*}
holds \emph{deterministically}.
Using the result~\eqref{eq:noise_bound}, we have
\begin{align}\label{eq:uncertainty_2}
    \mathbb P_2\left[
    \lvert f(x)-\mu_t(x)\rvert \leq
(
\|f\|_k+2\ln\left(
    \sqrt{
\det((1+\eta)I)+K_{t}
    }
    /\delta
    \right)
    ) 
    \cdot \sigma_t(x)
    \right] \geq 1-\delta.
\end{align}
Note that we might leave out a few constant factors for simplicity's sake to explain the problem of the probability spaces.

Now, we have seen that Uncertainty~\emph{(ii)} is not directly induced by the confidence intervals; it is introduced by the measurement noise.
Therefore, we do not need the independence of the RKHS norm over-estimation from the confidence intervals but we require the independence between the RKHS norm over-estimation from the probabilistic bound on the normed noise bound~\eqref{eq:noise_bound}.

Recall our Assumption~\ref{asm:random}, which states that:
\begin{quote}
% For any iteration~$t\geq 1$, given~$a_{1:t}, y_{1:t}$, the random RKHS functions~$\rho_{t,j}, j \in \{1, \ldots, m\}$, and the reward function~$f$ are i.i.d.\ samples from the same probability space.
\emph{For any iteration~$t\geq 1$, given~$a_{1:t}, y_{1:t}$, the RKHS norms of the random RKHS functions~$\|\rho_{t,j}\|_k, j \in \{1, \ldots, \mathrm m\}$, and the RKHS norm of the reward function~$\|f\|_k$ are i.i.d.\ samples from the same---potentially unknown---probability space.}
\end{quote}

To only way to directly combine the bounds~\eqref{eq:noise_bound} and~\eqref{eq:uncertainty_2} is to assume that we can fully separate aleatoric from epistemic uncertainty, \ie that the noisiness on the samples does not influence Assumption~\ref{asm:chow}.
Clearly, this assumption would be questionable since, \eg unbounded measurement noise would give us quite useless data to formulate random RKHS functions that resemble the ground truth.

However, if this assumption were sensible, we could formulate a classic product probability space with probability measure~$\tilde{\mathbb P} \coloneqq \mathbb P^m \otimes \mathbb P_2$, which yields
\begin{align*}
    \tilde{\mathbb P}\left[
    \lvert f(x)-\mu_t(x)\rvert \leq
(
\|f\|_k+2\ln\left(
    \sqrt{
\det((1+\eta)I)+K_{t}
    }
    /\delta
    \right)
    ) 
    \cdot \sigma_t(x)
    \right] \geq (1-\delta)(1-\gamma).
\end{align*}
Then, the safety guarantees would be with respect to the probability measure~$\tilde{\mathbb P}$.

\subsection{Joint instead of product probability spaces}
The idea would be to directly derive both probabilities in a joint probability space with joint probability measure~$\tilde{\mathbb P}$.
That is, we do not separately derive Uncertainty~\emph{(i)} with probability measure~$\mathbb P_1^m$ (scenario approach, uncertainty on random RKHS functions) and Uncertainty~\emph{(ii)} with probability measure~$\mathbb P_2$ (sub-Gaussian measurement noise, following \cite{chowdhury2017kernelized} or \cite{abbasi2013online}).

The joint probability space is very unrealistic. 
We assume that the probability space is not given so it makes no sense to create one by hand.

\subsection{Why a product probability space might be fine}

Problems for the story? 
We say that the probability space itself is unknown and we use the samples to generate it. In that ``macro''-sense, the probability space \emph{does} depend on the samples because we condition on them.
The way we implement it is that the given samples imply the deterministic part of the random RKHS functions. 
The stochasticity in the way we introduce in this paper does not depend on the samples. The stochasticity only comes from the tail coefficients and tail center points.
We can introduce it in this way for sure.
Then the RKHS norm is a transformation of the random variables (tail coefficients).

The story may be a little harmed by this because it again restricts the probability space by restricting the uncertainty to the tail variables.

But the RKHS norm depends on the (noisy) samples. It is a random variable. Can we separate it by introducing it like this?
